# Supplementary material for: Split Deep Q-Learning for Robust Object Singulation
Source: arXiv:1909.08105 source file (2020-02-27)
Supplement: Supplementary file 1 [file appendix.tex]

\appendix
Environment parameters (how many obstacles etc)

DQN parameters (learning rates etc)
